# Supplementary material for: Theoretical evidence for unexpected O-rich phases at corners of MgO surfaces
Source: arXiv:1706.05695 source file (2017-06-18)
Supplement: Supplementary file 1 [file SI-min.pdf]

# Theoretical evidence for unexpected O-rich phases at corners of MgO surfaces

Saswata Bhattacharya<sup>1</sup>, Daniel Berger<sup>2</sup>, Karsten Reuter<sup>2</sup>, L. M. Ghiringhelli<sup>3</sup>, Sergey V. Levchenko<sup>3</sup>

<sup>1</sup>*Indian Institute of Technology Delhi, Hauz Khas, New Delhi 110016, India*

<sup>2</sup>*Chair for Theoretical Chemistry and Catalysis Research Center,  
Technical University Munich, Lichtenbergstr. 4, D-85747 Garching, Germany*

<sup>3</sup>*Fritz-Haber-Institut der Max-Planck-Gesellschaft, Faradayweg 4-6, D-14195 Berlin, Germany*

(Dated: June 17, 2017)

## Supplemental Material

- I.** Different types of embedded MgO corners
- II.** Convergence of  $4\times 4\times 2@8\times 8\times 2$  size for the periodic model
- III.** Validation of QM/MM model calculations w.r.t periodic boundary calculations
- IV.** Phase diagrams for unembedded clusters
- V.** Concentration of defects and error estimation for  $\mu_e=\pm 0.2$  eV

## I. Different types of embedded MgO corners

We have generated different types of embedded model clusters. Some of them are shown below. The convergence of size of the QM region by varying the no. of atoms is tested as well.

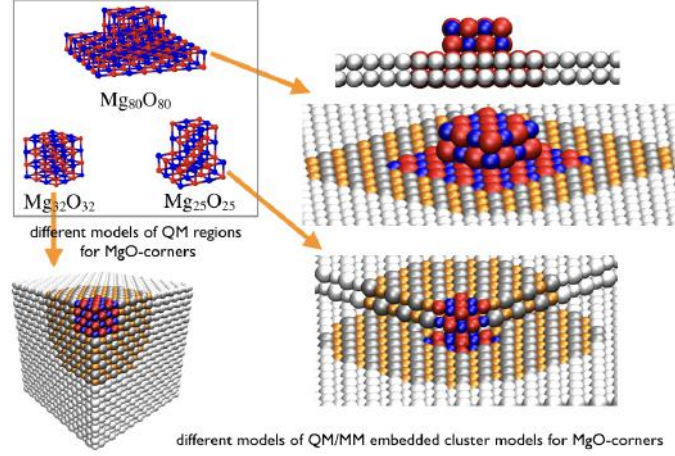

FIG. 1: Different types of embedded model clusters

## II. Convergence of $4 \times 4 \times 2 @ 8 \times 8 \times 2$ size for the periodic model

In order to validate our embedded model corner defect calculation w.r.t. periodic corner calculations, we have first created a periodic corner model. A  $4 \times 4 \times 2$  slab is placed on top of  $8 \times 8 \times 2$  slab. The size of the top slab (i.e.  $4 \times 4 \times 2$ ) as well as the bottom slab (i.e.  $8 \times 8 \times 2$ ) is converged by increasing the respective sizes. The resemblance in density of states confirms us the convergence of  $4 \times 4 \times 2 @ 8 \times 8 \times 2$  size for the periodic model calculations.

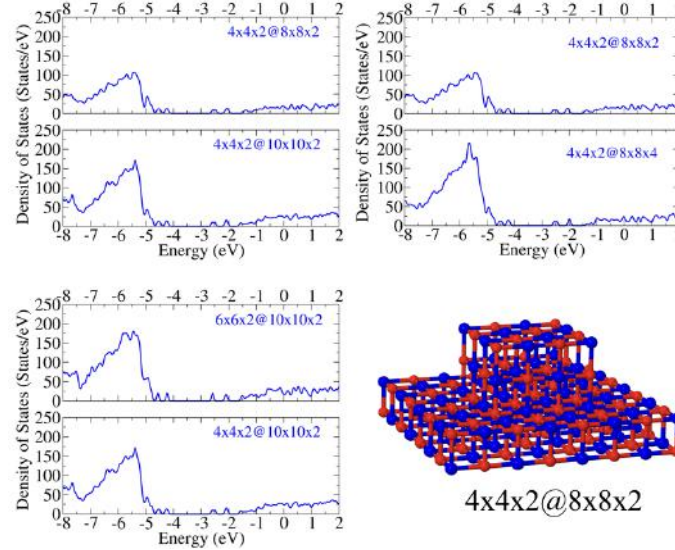

FIG. 2: Density of states of the respective periodic models at different sizes. The converged size of  $4 \times 4 \times 2 @ 8 \times 8 \times 2$  slab is shown.

## III. Validation of QM/MM model calculations w.r.t periodic boundary calculations

For an accurate description of defect charging, the embedding scheme should closely reproduce the electronic structure of the corresponding extended system, in particular the position of the defect levels w.r.t the bulk Fermi level. We check this by comparing the electronic structure of the embedded cluster model of an unmodified O-terminated corner with a periodic slab model (i.e.  $4 \times 4 \times 2 @ 8 \times 8 \times 2$  slab as described above). Since we focus on *p*-doped MgO, the Fermi level is set to the valence band maximum (VBM). The position of the highest occupied state (HOMO) for the corner defect w.r.t the bulk Fermi level is determined as follows. First, the position of the Fermi level w.r.t the vacuum

level is calculated using the HSE06 functional. This is done by calculating the position of the Mg 1s core state in the third layer of a 5-layer MgO (100) slab w.r.t vacuum. By aligning the positions of the Mg 1s core states in the slab and in the bulk, the position of the VBM w.r.t vacuum is then calculated. The result is -7.5 eV. Next, the position of the HOMO w.r.t vacuum is calculated from the embedded cluster model. To ensure that no artificial shift of the HOMO relative to the vacuum level is induced by the embedding, we compare the positions of the HOMO for both the embedded cluster and the periodic slab models of the pristine neutral corner, calculated with the PBE [? ? ] functional. The periodic model was converged in terms of the number of layers and lateral dimensions. The resulting difference is found to be about 0.2 eV. We conclude that we have an uncertainty of at most  $\pm 0.2$  eV (depending on the type of corner) in the position of the defect levels w.r.t the Fermi level due to embedding.

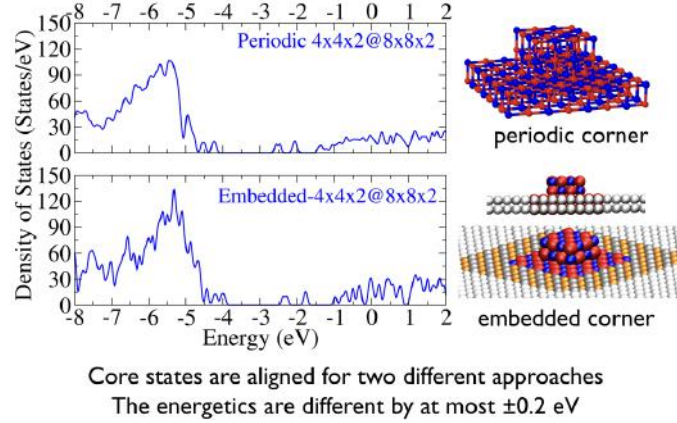

FIG. 3: Density of states for the defect level using two different approaches viz. periodic calculations (top) and embedded-cluster model (bottom).

## IV. Phase diagrams for unembedded clusters

We have tried to understand the relative stability of a set of medium-size parallelepipedal  $[\text{Mg}_N\text{O}_{(x+N)}]^q$  clusters at various sizes  $[N = 18, 24, 32, 108]$  with a defect at one of the corners  $[x = -1(\text{O-vacancy}), 0(\text{pristine}), 1(\text{O-ad-species}), 2(\text{O}_2\text{-ad-species})]$ . The charge states  $q$  is varied from -2 to +2  $[q = -2, -1, 0, 1, 2]$ . Note that using our massively-parallel cascade genetic algorithm implementation [cGA], we have noticed that the corners of such parallelepipedal clusters, are the most active sites to create defects. Therefore, globally optimized structures of  $[\text{Mg}_N\text{O}_{(x+N)}]^q$  clusters are generated by means of our cGA implementation. We find that at a realistic temperatures and pressures (e.g.,  $T = 300\text{K}$ ,  $p_{\text{O}_2} \sim 1 \text{ atm}$ ) O or  $\text{O}_2$ -interstitial states at the oxygen corners of pristine  $[(\text{MgO})_N]^q$  clusters are favored at all studied charge states, over a wide range of electronic chemical potential  $\mu_e$ . In fact, the interstitials are stable even at some values of  $\mu_e$ , for which O-vacancies are preferred at flat (100) surfaces of doped MgO. Strikingly, this behaviour is also confirmed when some model clusters are embedded in a point-charge array, in order to mimic the realization of a corner defect (intersection of two step ridges) on an extended surface as shown in the main manuscript or the case embedded- $(\text{MgO})_{25+x}^q$  below:

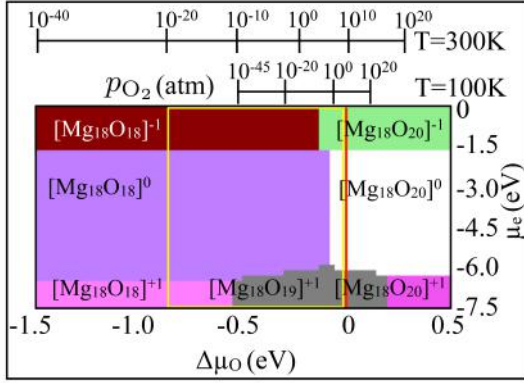

(a)  $(\text{MgO})_{18+x}^q$

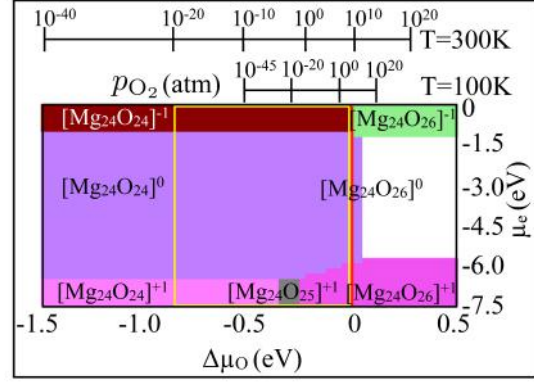

(b)  $(\text{MgO})_{24+x}^q$

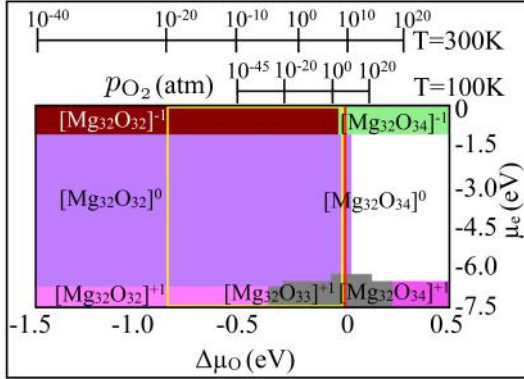

(c)  $(\text{MgO})_{32+x}^q$

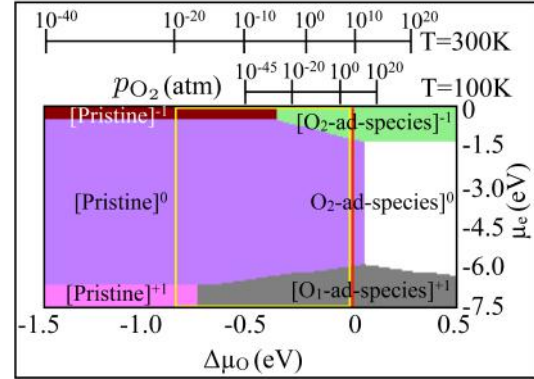

(d) embedded- $(\text{MgO})_{25+x}^q$

## V. Concentration of defects and error estimation for $\mu_e = \pm 0.2$ eV

Following figure shows the concentration of different kinds of defects at varying temperature and constant pressure. As it can be seen from comparing the concentrations of various kind of defects at different pressures, the estimated error of  $\pm 0.2$  eV in the position of the defect levels w.r.t the electronic chemical potential has no qualitative effect on the calculated relative concentrations.

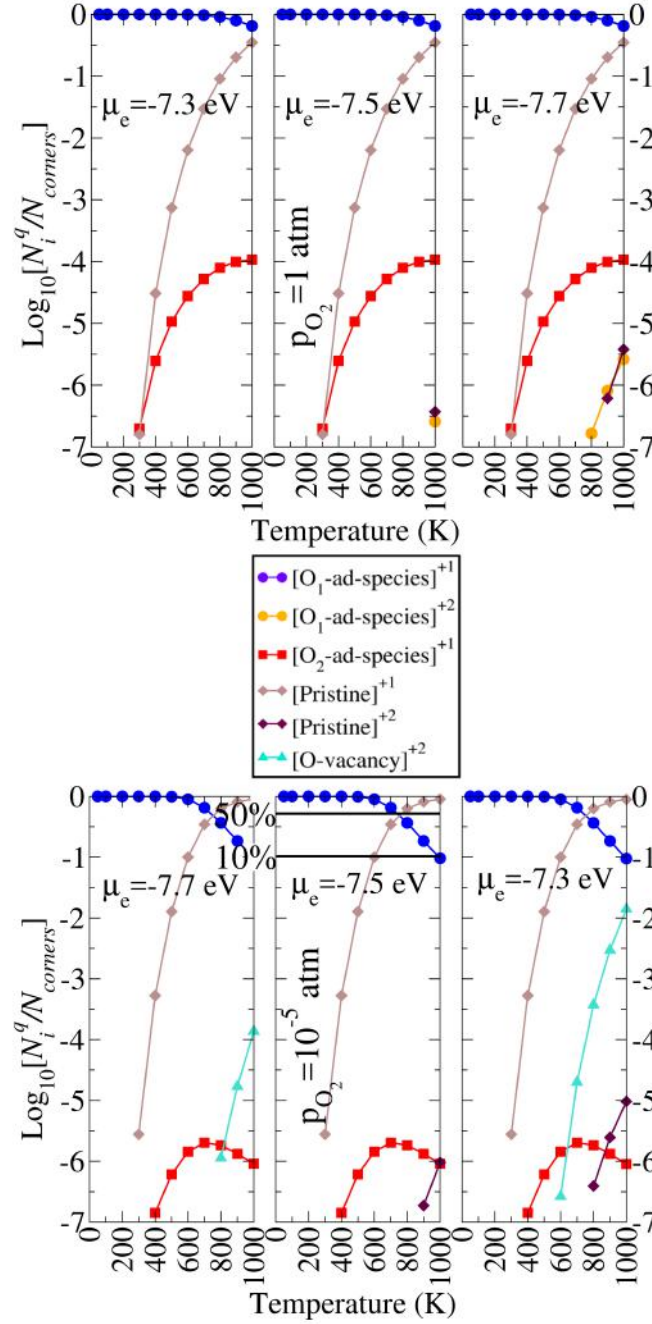

FIG. 4: Concentration of defect at  $p_{O_2} = 1$  atm and  $p_{O_2} = 10^{-5}$  atm.
